# Supplementary material for: Domain Generalization via Contrastive Causal Learning
Source: arXiv:2210.02655 source file (2022-10-06)
Supplement: Supplementary file 1 [file appendix.tex]

\clearpage
\appendix

\setcounter{secnumdepth}{2}
\setcounter{table}{0}
\setcounter{figure}{0}

\section{Detailed Results}
\label{appendix}
In this section, the Table\ref{tab:PACS}, Table \ref{tab:OfficeHome}, and Table \ref{tab:TerraIncognita} show that CCM has more balanced results in each domain with high average values.And the ablation studies are shown in Table \ref{tab:ablation_PACS}, Table \ref{tab:ablation_OfficeHome}, and Table \ref{tab:ablation_TerraIncognita}. We can find that CCM exhibits a significant drop in performance which means CCM needs $L_{teach}$ to obtain the basic correlation knowledge. With the help of $L_{learn}$ and $L_{self}$, CCM increases the percentage of true causal effects to improve accuracy via the front-door criterion.

% \subsection{Accuracy}
\begin{table}[ht]
    \centering
    \adjustbox{max width=\linewidth}{%
    \begin{tabular}{lccccc}
    \toprule
    \textbf{Algorithm}   & \textbf{A}           & \textbf{C}           & \textbf{P}           & \textbf{S}           & \textbf{Avg}         \\
    \midrule
    ERM                  & 84.7 $\pm$ 0.4       & \underline{80.8 $\pm$ 0.6}       & 97.2 $\pm$ 0.3       & 79.3 $\pm$ 1.0       & 85.5                 \\
    IRM                  & 84.8 $\pm$ 1.3       & 76.4 $\pm$ 1.1       & 96.7 $\pm$ 0.6       & 76.1 $\pm$ 1.0       & 83.5                 \\
    GroupDRO             & 83.5 $\pm$ 0.9       & 79.1 $\pm$ 0.6       & 96.7 $\pm$ 0.3       & 78.3 $\pm$ 2.0       & 84.4                 \\
    Mixup                & 86.1 $\pm$ 0.5       & 78.9 $\pm$ 0.8       & \textbf{97.6 $\pm$ 0.1}       & 75.8 $\pm$ 1.8       & 84.6                 \\
    MLDG                 & 85.5 $\pm$ 1.4       & 80.1 $\pm$ 1.7       & 97.4 $\pm$ 0.3       & 76.6 $\pm$ 1.1       & 84.9                 \\
    CORAL                & 88.3 $\pm$ 0.2       & 80.0 $\pm$ 0.5       & 97.5 $\pm$ 0.3       & 78.8 $\pm$ 1.3       & 86.2                 \\
    MMD                  & 86.1 $\pm$ 1.4       & 79.4 $\pm$ 0.9       & 96.6 $\pm$ 0.2       & 76.5 $\pm$ 0.5       & 84.6                 \\
    DANN                 & 86.4 $\pm$ 0.8       & 77.4 $\pm$ 0.8       & 97.3 $\pm$ 0.4       & 73.5 $\pm$ 2.3       & 83.6                 \\
    CDANN                & 84.6 $\pm$ 1.8       & 75.5 $\pm$ 0.9       & 96.8 $\pm$ 0.3       & 73.5 $\pm$ 0.6       & 82.6                 \\
    MTL                  & 87.5 $\pm$ 0.8       & 77.1 $\pm$ 0.5       & 96.4 $\pm$ 0.8       & 77.3 $\pm$ 1.8       & 84.6                 \\
    SagNet               & 87.4 $\pm$ 1.0       & 80.7 $\pm$ 0.6       & 97.1 $\pm$ 0.1       & \underline{80.0 $\pm$ 0.4}       & \underline{86.3}     \\
    ARM                  & 86.8 $\pm$ 0.6       & 76.8 $\pm$ 0.5       & 97.4 $\pm$ 0.3       & 79.3 $\pm$ 1.2       & 85.1                 \\
    VREx                 & 86.0 $\pm$ 1.6       & 79.1 $\pm$ 0.6       & 96.9 $\pm$ 0.5       & 77.7 $\pm$ 1.7       & 84.9                 \\
    RSC                  & 85.4 $\pm$ 0.8       & 79.7 $\pm$ 1.8       & \underline{97.6 $\pm$ 0.3}       & 78.2 $\pm$ 1.2       & 85.2                 \\
    SAND-mask            & 85.8 $\pm$ 1.7       & 79.2 $\pm$ 0.8       & 96.3 $\pm$ 0.2       & 76.9 $\pm$ 2.0       & 84.6                 \\
    Fishr                & \underline{88.4 $\pm$ 0.2}       & 78.7 $\pm$ 0.7       & 97.0 $\pm$ 0.1       & 77.8 $\pm$ 2.0       & 85.5                 \\
    \midrule
    CCM                  & \textbf{88.6 $\pm$ 0.4}       & \textbf{82.0 $\pm$ 0.5}       & 97.0 $\pm$ 0.5       & \textbf{80.2 $\pm$ 0.5}       & \textbf{87.0}        \\
    \bottomrule
    \end{tabular}}
    \caption{Domain generalization results of category classification on PACS.}
    \label{tab:PACS}
\end{table}

\begin{table}[ht]
    \centering
    \adjustbox{max width=\linewidth}{%
    \begin{tabular}{lccccc}
    \toprule
    \textbf{Algorithm}   & \textbf{A}           & \textbf{C}           & \textbf{P}           & \textbf{R}           & \textbf{Avg}         \\
    \midrule
    ERM                  & 61.3 $\pm$ 0.7       & 52.4 $\pm$ 0.3       & 75.8 $\pm$ 0.1       & 76.6 $\pm$ 0.3       & 66.5                 \\
    IRM                  & 58.9 $\pm$ 2.3       & 52.2 $\pm$ 1.6       & 72.1 $\pm$ 2.9       & 74.0 $\pm$ 2.5       & 64.3                 \\
    GroupDRO             & 60.4 $\pm$ 0.7       & 52.7 $\pm$ 1.0       & 75.0 $\pm$ 0.7       & 76.0 $\pm$ 0.7       & 66.0                 \\
    Mixup                & 62.4 $\pm$ 0.8       & 54.8 $\pm$ 0.6       & \underline{76.9 $\pm$ 0.3}       & 78.3 $\pm$ 0.2       & 68.1                 \\
    MLDG                 & 61.5 $\pm$ 0.9       & 53.2 $\pm$ 0.6       & 75.0 $\pm$ 1.2       & 77.5 $\pm$ 0.4       & 66.8                 \\
    CORAL                & \textbf{65.3 $\pm$ 0.4}       & 54.4 $\pm$ 0.5       & 76.5 $\pm$ 0.1       & \underline{78.4 $\pm$ 0.5}       & \underline{68.7}                 \\
    MMD                  & 60.4 $\pm$ 0.2       & 53.3 $\pm$ 0.3       & 74.3 $\pm$ 0.1       & 77.4 $\pm$ 0.6       & 66.3                 \\
    DANN                 & 59.9 $\pm$ 1.3       & 53.0 $\pm$ 0.3       & 73.6 $\pm$ 0.7       & 76.9 $\pm$ 0.5       & 65.9                 \\
    CDANN                & 61.5 $\pm$ 1.4       & 50.4 $\pm$ 2.4       & 74.4 $\pm$ 0.9       & 76.6 $\pm$ 0.8       & 65.8                 \\
    MTL                  & 61.5 $\pm$ 0.7       & 52.4 $\pm$ 0.6       & 74.9 $\pm$ 0.4       & 76.8 $\pm$ 0.4       & 66.4                 \\
    SagNet               & 63.4 $\pm$ 0.2       & \underline{54.8 $\pm$ 0.4}       & 75.8 $\pm$ 0.4       & 78.3 $\pm$ 0.3       & 68.1                 \\
    ARM                  & 58.9 $\pm$ 0.8       & 51.0 $\pm$ 0.5       & 74.1 $\pm$ 0.1       & 75.2 $\pm$ 0.3       & 64.8                 \\
    VREx                 & 60.7 $\pm$ 0.9       & 53.0 $\pm$ 0.9       & 75.3 $\pm$ 0.1       & 76.6 $\pm$ 0.5       & 66.4                 \\
    RSC                  & 60.7 $\pm$ 1.4       & 51.4 $\pm$ 0.3       & 74.8 $\pm$ 1.1       & 75.1 $\pm$ 1.3       & 65.5                 \\
    SAND-mask            & 60.3 $\pm$ 0.5       & 53.3 $\pm$ 0.7       & 73.5 $\pm$ 0.7       & 76.2 $\pm$ 0.3       & 65.8                 \\
    Fishr                & 62.4 $\pm$ 0.5       & 54.4 $\pm$ 0.4       & 76.2 $\pm$ 0.5       & 78.3 $\pm$ 0.1       & 67.8                 \\
    \midrule
    CCM                  & \underline{64.9 $\pm$ 0.5}   & \textbf{56.7 $\pm$ 0.3}    & \textbf{78.1 $\pm$ 0.1}   & \textbf{79.0 $\pm$ 0.7}   & \textbf{69.7}        \\
    \bottomrule
    \end{tabular}}
    \caption{Domain generalization results of category classification on OfficeHome.}
    \label{tab:OfficeHome}
\end{table}

\begin{table}[ht]
    \centering
    \adjustbox{max width=\linewidth}{%
    \begin{tabular}{lccccc}
    \toprule
    \textbf{Algorithm}   & \textbf{L100}        & \textbf{L38}         & \textbf{L43}         & \textbf{L46}         & \textbf{Avg}         \\
    \midrule
    ERM                  & 49.8 $\pm$ 4.4       & 42.1 $\pm$ 1.4       & 56.9 $\pm$ 1.8       & 35.7 $\pm$ 3.9       & 46.1                 \\
    IRM                  & 54.6 $\pm$ 1.3       & 39.8 $\pm$ 1.9       & 56.2 $\pm$ 1.8       & 39.6 $\pm$ 0.8       & 47.6                 \\
    GroupDRO             & 41.2 $\pm$ 0.7       & 38.6 $\pm$ 2.1       & 56.7 $\pm$ 0.9       & 36.4 $\pm$ 2.1       & 43.2                 \\
    Mixup                & \textbf{59.6 $\pm$ 2.0}       & 42.2 $\pm$ 1.4       & 55.9 $\pm$ 0.8       & 33.9 $\pm$ 1.4       & \underline{47.9}                 \\
    MLDG                 & 54.2 $\pm$ 3.0       & \textbf{44.3 $\pm$ 1.1}       & 55.6 $\pm$ 0.3       & 36.9 $\pm$ 2.2       & 47.7                 \\
    CORAL                & 51.6 $\pm$ 2.4       & 42.2 $\pm$ 1.0       & 57.0 $\pm$ 1.0       & 39.8 $\pm$ 2.9       & 47.6                 \\
    MMD                  & 41.9 $\pm$ 3.0       & 34.8 $\pm$ 1.0       & 57.0 $\pm$ 1.9       & 35.2 $\pm$ 1.8       & 42.2                 \\
    DANN                 & 51.1 $\pm$ 3.5       & 40.6 $\pm$ 0.6       & 57.4 $\pm$ 0.5       & 37.7 $\pm$ 1.8       & 46.7                 \\
    CDANN                & 47.0 $\pm$ 1.9       & 41.3 $\pm$ 4.8       & 54.9 $\pm$ 1.7       & 39.8 $\pm$ 2.3       & 45.8                 \\
    MTL                  & 49.3 $\pm$ 1.2       & 39.6 $\pm$ 6.3       & 55.6 $\pm$ 1.1       & 37.8 $\pm$ 0.8       & 45.6                 \\
    SagNet               & 53.0 $\pm$ 2.9       & 43.0 $\pm$ 2.5       & \textbf{57.9 $\pm$ 0.6}       & 40.4 $\pm$ 1.3       & \textbf{48.6}                 \\
    ARM                  & 49.3 $\pm$ 0.7       & 38.3 $\pm$ 2.4       & 55.8 $\pm$ 0.8       & 38.7 $\pm$ 1.3       & 45.5                 \\
    VREx                 & 48.2 $\pm$ 4.3       & 41.7 $\pm$ 1.3       & 56.8 $\pm$ 0.8       & 38.7 $\pm$ 3.1       & 46.4                 \\
    RSC                  & 50.2 $\pm$ 2.2       & 39.2 $\pm$ 1.4       & 56.3 $\pm$ 1.4       & \textbf{40.8 $\pm$ 0.6}       & 46.6                 \\
    SAND-mask            & 45.7 $\pm$ 2.9       & 31.6 $\pm$ 4.7       & 55.1 $\pm$ 1.0       & 39.0 $\pm$ 1.8       & 42.9                 \\
    Fishr                & 50.2 $\pm$ 3.9       & \underline{43.9 $\pm$ 0.8}       & \underline{55.7 $\pm$ 2.2}       & \underline{39.8 $\pm$ 1.0}       & 47.4 \\
    % \hline
    \midrule
    CCM                  & \underline{56.6 $\pm$ 0.8}       & 42.9 $\pm$ 2.0       & 57.3 $\pm$ 0.7       & 37.5 $\pm$ 0.3       & \textbf{48.6}                 \\
    \bottomrule
    \end{tabular}}
    \caption{Domain generalization results of category classification on TerraIncognita.}
    \label{tab:TerraIncognita}
\end{table}

% \subsection{Ablation Study}
\begin{table}[ht]
    \centering
    \adjustbox{max width=\linewidth}{%
    \begin{tabular}{lccccc}
    \toprule
    \textbf{Algorithm}  & \textbf{A}           & \textbf{C}           & \textbf{P}           & \textbf{S}           & \textbf{Avg}  \\
    \midrule
    ERM                             & 84.7      & 80.8      & 97.2       & 79.3      & 85.5 \\
    \midrule
    CCM w/o  $\mathcal{L}_{teach}$  & 18.7      & 20.7      & 12.4       & 19.1      & 17.7 \\
    CCM w/o  $\mathcal{L}_{learn}$  & 87.3      & 79.1      & 97.1       & 80.8      & 86.1 \\
    CCM w/o  $\mathcal{L}_{self}$   & 87.1  & 83.6  & 97.0 & 78.2  & 86.5 \\
    CCM w  $\mathcal{L}_{teach}$    & 85.8  & 82.6  & 97.3 & 79.0  & 86.2 \\
    CCM                             & 88.6  & 82.0  & 97.0 & 80.2  & 87.0 \\
    \bottomrule
    \end{tabular}}
    \caption{Ablation study results of $\mathcal{L}_{teach}$, $\mathcal{L}_{learn}$ and $\mathcal{L}_{self}$ on PACS.}
    \label{tab:ablation_PACS}
\end{table}

\begin{table}[ht]
    \centering
    \adjustbox{max width=\linewidth}{%
    \begin{tabular}{lccccc}
    \toprule
    \textbf{Algorithm}  & \textbf{A}           & \textbf{C}           & \textbf{P}           & \textbf{R}           & \textbf{Avg}  \\
    \midrule
    ERM                             & 61.3       & 52.4       & 75.8       & 76.6       & 66.5 \\
    \midrule
    CCM w/o  $\mathcal{L}_{teach}$  & 0.7       & 2.3      & 1.0       & 1.7      & 1.4 \\
    CCM w/o  $\mathcal{L}_{learn}$  & 64.0      & 57.2      & 78.4       & 79.1      & 69.7 \\
    CCM w/o  $\mathcal{L}_{self}$   & 63.3  & 56.3  & 77.9 & 79.4  & 69.3 \\
    CCM w  $\mathcal{L}_{teach}$    & 63.6  & 56.7  & 78.0 & 79.0  & 69.3 \\
    CCM                             & 64.9  &  56.7  & 78.1 & 79.0   & 69.7 \\
    \bottomrule
    \end{tabular}}
    \caption{Ablation study results of $\mathcal{L}_{teach}$, $\mathcal{L}_{learn}$ and $\mathcal{L}_{self}$ on OfficeHome.}
    \label{tab:ablation_OfficeHome}
\end{table}

\begin{table}[ht]
    \centering
    \adjustbox{max width=\linewidth}{%
    \begin{tabular}{lccccc}
    \toprule
    \textbf{Algorithm}  & \textbf{L100}        & \textbf{L38}         & \textbf{L43}         & \textbf{L46}         & \textbf{Avg}  \\
    \midrule
    ERM                  & 49.8       & 42.1       & 56.9       & 35.7       & 46.1 \\
    \midrule
    CCM w/o  $\mathcal{L}_{teach}$  & 20.0      & 2.0       & 18.6       & 18.7      & 14.8 \\
    CCM w/o  $\mathcal{L}_{learn}$  & 53.8      & 44.2      & 55.9       & 39.6      & 48.4 \\
    CCM w/o  $\mathcal{L}_{self}$   & 56.7  & 43.2  & 56.4 & 39.1  & 48.8 \\
    CCM w  $\mathcal{L}_{teach}$    & 52.7  & 43.1  & 56.0 & 37.1  & 47.2 \\
    CCM                             & 56.6  & 42.9  & 57.3 & 37.5  & 48.6 \\
    \bottomrule
    \end{tabular}}
    \caption{Ablation study results of $\mathcal{L}_{teach}$, $\mathcal{L}_{learn}$ and $\mathcal{L}_{self}$ on TerraIncognita.}
    \label{tab:ablation_TerraIncognita}
\end{table}
